# Supplementary material for: Self-supervised Video Representation Learning with Motion-Aware Masked Autoencoders
Source: arXiv:2210.04154 source file (2022-10-09)
Supplement: Supplementary file 2 [file finetune_schedule_supp.tex]

\begin{table}[t]
\centering
\begin{tabular}{c}
Epoch & Repeat Aug. & topp-1(\%) \\
\shline \hline
20 & w/o & 74.0 \\
30 & w/o & 74.5 \\
40 & w/o & 74.2 \\
20 & w/ & 74.6 \\

\end{tabular}
\caption{xxxx
}
\label{tab:vos}
\end{table}
